# Supplementary material for: Boosting as Frank-Wolfe
Source: arXiv:2209.10831 source file (2022-09-30)
Supplement: Supplementary file 1 [file fenchel_duality.tex]

\section{Fenchel duality review}
\label{appendix:fenchel_duality}
First, we introduce some additional notations.
For a function $f : \mathbb{R}^m \to (-\infty, +\infty]$, 
let $\domain f = \{ \bm{d} | f(\bm{d}) < +\infty \}$. 
For a convex set $C \subset \mathbb{R}^n$, 
define the set of interior points $\interior(C)$ as
\begin{align*}
    \interior(C) = \{
        \bm{w} \in C \mid
            \forall \bm{d} \in \mathbb{R}^n,
            \exists t > 0,
            \forall \tau \in [0, t], \bm{w} + \tau \bm{d} \in C
    \}.
\end{align*}
For sets $A$ and $B$ over $\mathbb R^n$, 
define $A - B = \{ \bm{a} - \bm{b} \mid \bm{a} \in A, \bm{b} \in B\}$. 

\begin{theorem}[\cite{borwein+:springer06}]
    \label{thm:appendix_strong_duality}
    Let $f : \mathbb{R}^m \to (-\infty, +\infty]$ and 
    $g : \mathbb{R}^n \to (-\infty, +\infty]$ be convex functions 
    and a linear map $M : \mathbb{R}^m \to \mathbb{R}^n$. 
    Define the Fenchel problems
    \begin{align}
        \label{eq:appendix_strong_duality_primal}
        \gamma & = \inf_{\bm{d}} f(\bm{d}) + g(M^\top\bm{d}), \\
        \label{eq:appendix_strong_duality_dual}
        \rho   & = \sup_{\bm{w}} -f^\star(-M \bm{w}) - g^\star(\bm{w}).
    \end{align}
    Then, $\gamma \geq \rho$ holds. Further, $\gamma = \rho$ holds if 
    \begin{align}
        \label{eq:appendix_strong_duality_qualification}
        \bm{0} \in 
        \interior
        \left(\domain g - M^\top \domain f\right).
    \end{align}
    Further, points $\bm{d}^\star \in \psimplex{m}_{\nu}$ and 
    $\bm{w}^\star \in \psimplex{n}$ are optimal solutions 
    for problems~(\ref{eq:appendix_strong_duality_primal}) 
    and~(\ref{eq:strong_duality_dual}), respectively, 
    if and only if $-M \bm{w}^\star \in \partial f(\bm{d}^\star)$ 
    and $\bm{w}^\star \in \partial g(M^\top \bm{d}^\star)$.
\end{theorem}
